# Supplementary material for: Stabilization of exponential number of discrete remanent states with localized spin-orbit torques
Source: arXiv:2005.10051 source file (2020-05-20)
Supplement: Supplementary file 1 [file Supplementary.pdf]

# Supplementary - Stabilization of exponential number of discrete remanent states with localized spin-orbit torques

Shubhankar Das, Ariel Zaig, Moty Schultz, and Lior Klein
*Department of Physics, Nano-magnetism Research Center,*
*Institute of Nanotechnology and Advanced Materials, Bar-Ilan University, Ramat-Gan 52900, Israel*
(Dated: April 26, 2020)

## I. On-off measurements

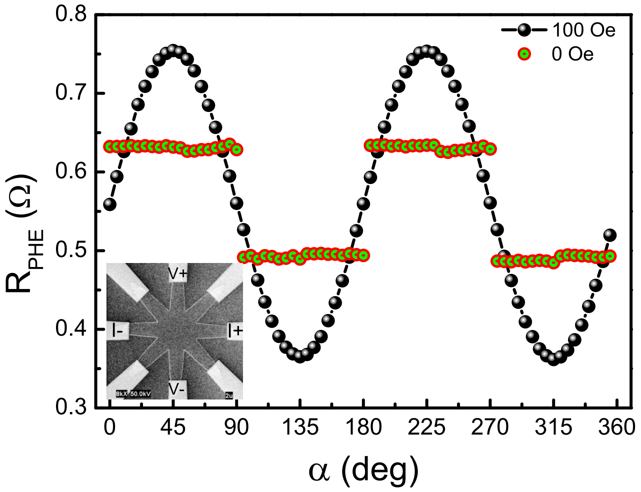


FIG. S1: $R_{PHE}$ vs $\alpha$ with a field of 100 Oe and after the field is removed for each $\alpha$. The current and voltage pads are shown in the inset.

Planar Hall resistance ($R_{PHE}$) is measured by flowing current in the horizontal ellipse and probing voltage across the vertical ellipse in a four crossing ellipses (4CE) structure (see the inset of Fig. S1). Fig. S1 shows $R_{PHE}$ as a function of angle between field and current direction ($\alpha$) and for each values of $\alpha$, $R_{PHE}$ is measured with a saturation field of 100 Oe and after the field is switched off. At remanent states we only observe two plateaus instead of four when voltage is measured across the slanted ellipses (see main text), because of the symmetry of the planar Hall effect.

### II. Reversible switchings between OSs in 4CE structure

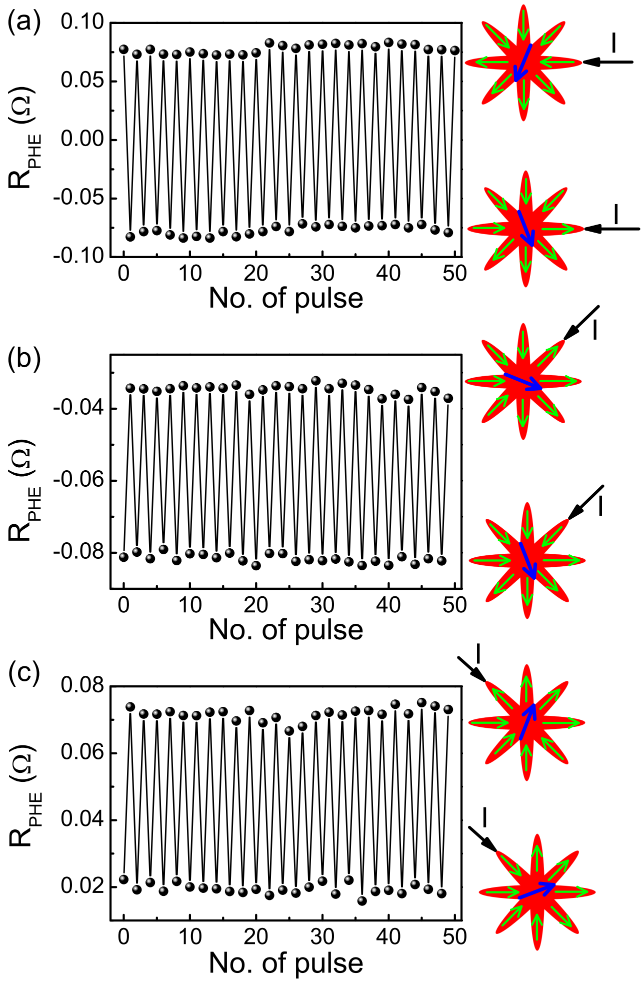


FIG. S2: (a), (b) and (c) Field-free reversible switchings between OSs by flowing current through individual ellipses. The direction of magnetization in the overlap area and edges of the OSs are shown by arrows.

Field-free reproducible reversible switchings (50 times) between ordinary states (OSs) are demonstrated in Fig. S2(a), (b) and (c) by flowing current through individual ellipses. Note that in the presented cases the reversible switchings are obtained by flowing current through the same ellipse and in same direction.

### III. Reversible switchings between OSs and SSs in 4CE structure

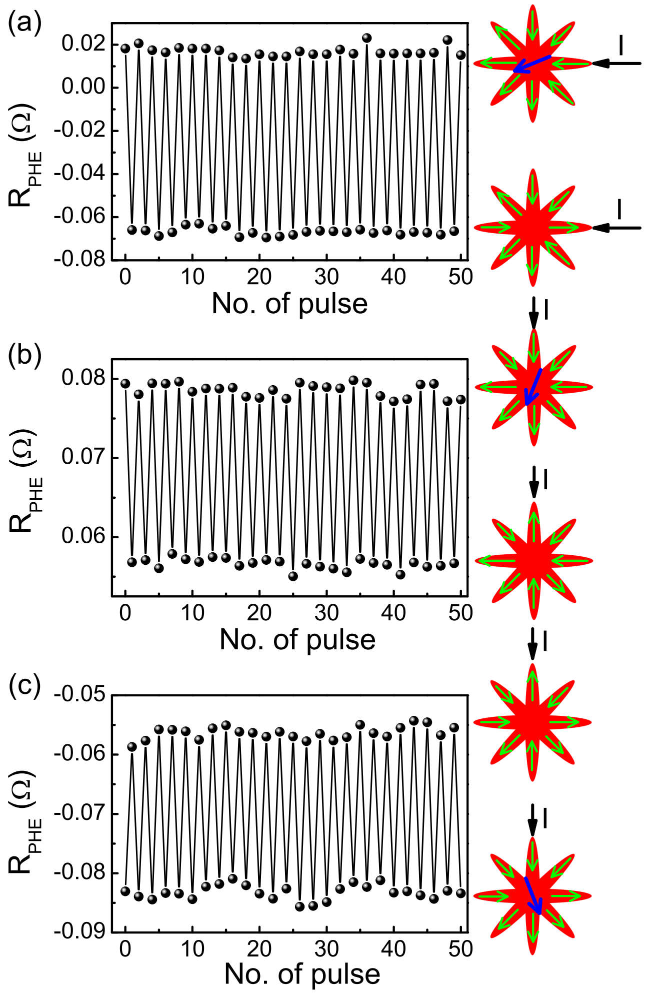


FIG. S3: (a), (b) and (c) Field-free reversible switchings between OSs and SSs by flowing current through individual ellipses. The direction of magnetization in the overlap area and edges of the remanent states are shown by arrows.

Field-free reversible switchings between OSs and staggered states (SSs) are demonstrates in Fig. S3 (a), (b) and (c) by flowing current in the same direction through individual ellipses. In all the switchings, we flow a current pulses of 2.5 mA through the same ellipse, followed by a small probing current of 50 $\mu$A to measure $R_{PHE}$.

## IV. Reversible switchings between OSs and SSs in 3CE structure

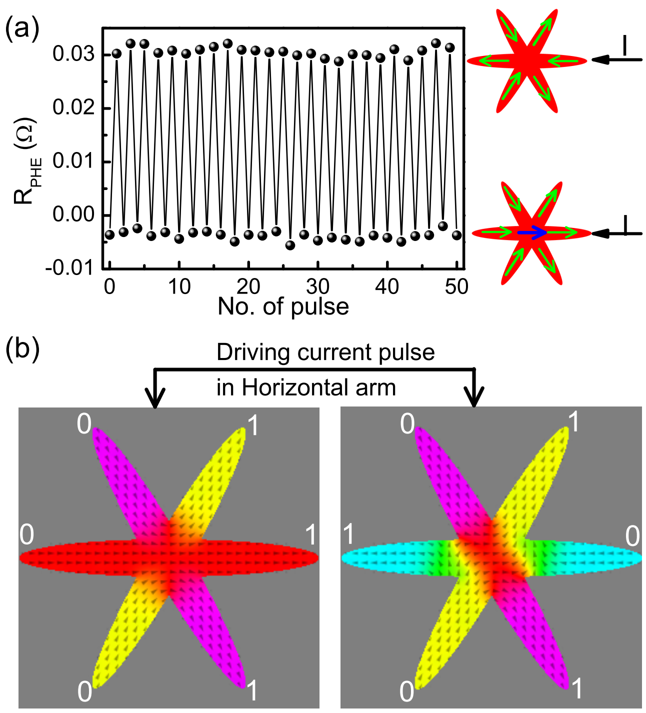


FIG. S4: (a) Field-free reversible switchings between OS and SS by flowing 50 current pulses of 2.5 mA through the horizontal arm. (b) Micro-magnetic simulation of switchings between an OS and a SS by driving a spin-polarized current pulse through the horizontal ellipse.

Here, we explore the stabilization of SSs in a three crossing ellipses (3CE) structure and switching between an OS and a SS. Fig. S4(a) shows reversible switchings between states by flowing 50 current pulses of amplitude 2.5 mA through the horizontal ellipse. The $R_{PHE}$ value of one of the states differ from the remanent values obtained when the states are stabilized by an external magnetic field (see Fig. 1(e) of main text). We identify this state as one of the SSs by numerical simulation of the $R_{PHE}$ value of the state and micromagnetic simulation. Fig. S4(b) shows simulated[1] switchings between an OS and a SS, where a spin-polarized current pulse of $6 \times 10^6$ A/cm$^2$ and duration 2 ns is driven in the horizontal ellipse of 3CE of dimension $2.048 \times 16.384$ $\mu$m$^2$ and thickness 2 nm. The other SS can also be achieved by driving an opposite current pulse in the horizontal arm of the reversed OS. We note that the $R_{PHE}$ value of the two SSs are identical.

## V. The remanent states in a 2CE structure

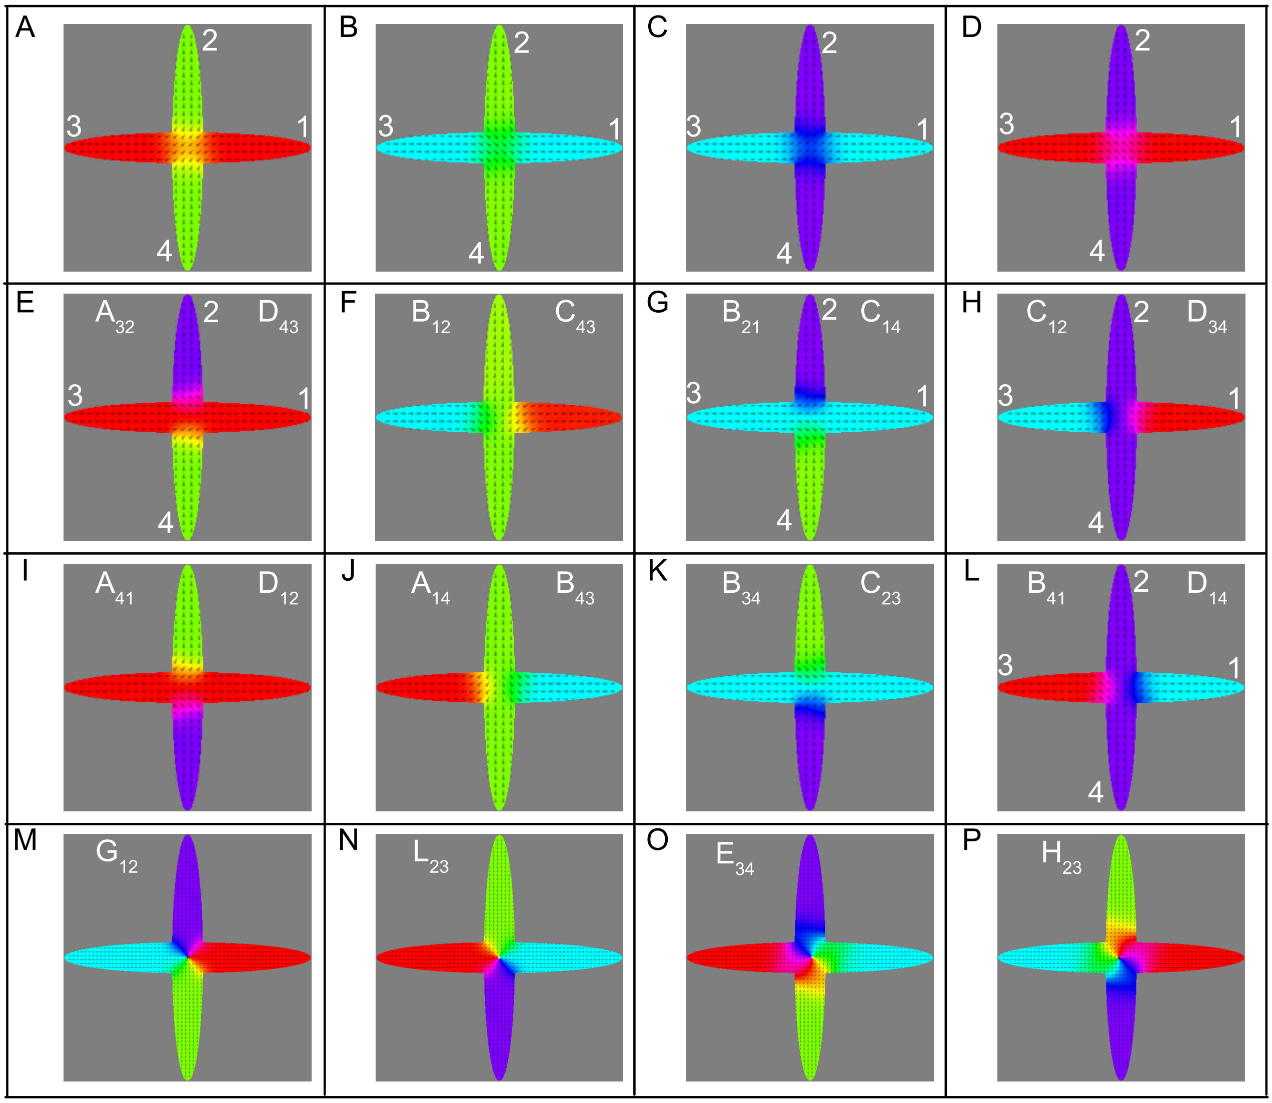


FIG. S5: The magnetic configurations of four ordinary states. The numbers denote the contact pads. (E-L) The magnetic configurations of eight $\pi$-Neel-type domain states. The abbreviations denote how the states can be achieved experimentally. See the text for details. (M-P) The magnetic configurations of four states, where for each of the 2 ellipses the magnetization points in opposite directions in its edges.

A 2CE structure supports $2^4$ remanent states. The magnetic configurations of the 16 states obtained by simulations are presented in Fig. S5. We can separate the 16 states into 3 groups:

Group 1 (Fig. S5(A)-(D)): 4 ordinary states where the magnetization in the edges of each ellipse points in the same direction.

Group 2 (Fig. S5(E)-(L)): 8 states where in one ellipse the magnetization points in the same direction in both edges whereas in the other ellipse the magnetization points in opposite directions in its edges.

Group 3 (Fig. S5(M)-(P)): 4 states where for each of the 2 ellipses the magnetization points in opposite directions in its edges.

In the main text we identify the states in Group 1 as OSs and the states in Group 2 and 3 as NSs.

The 4 states of Group 1 are clearly accessible by applying and removing an external field as shown in Fig. 1(d) of main

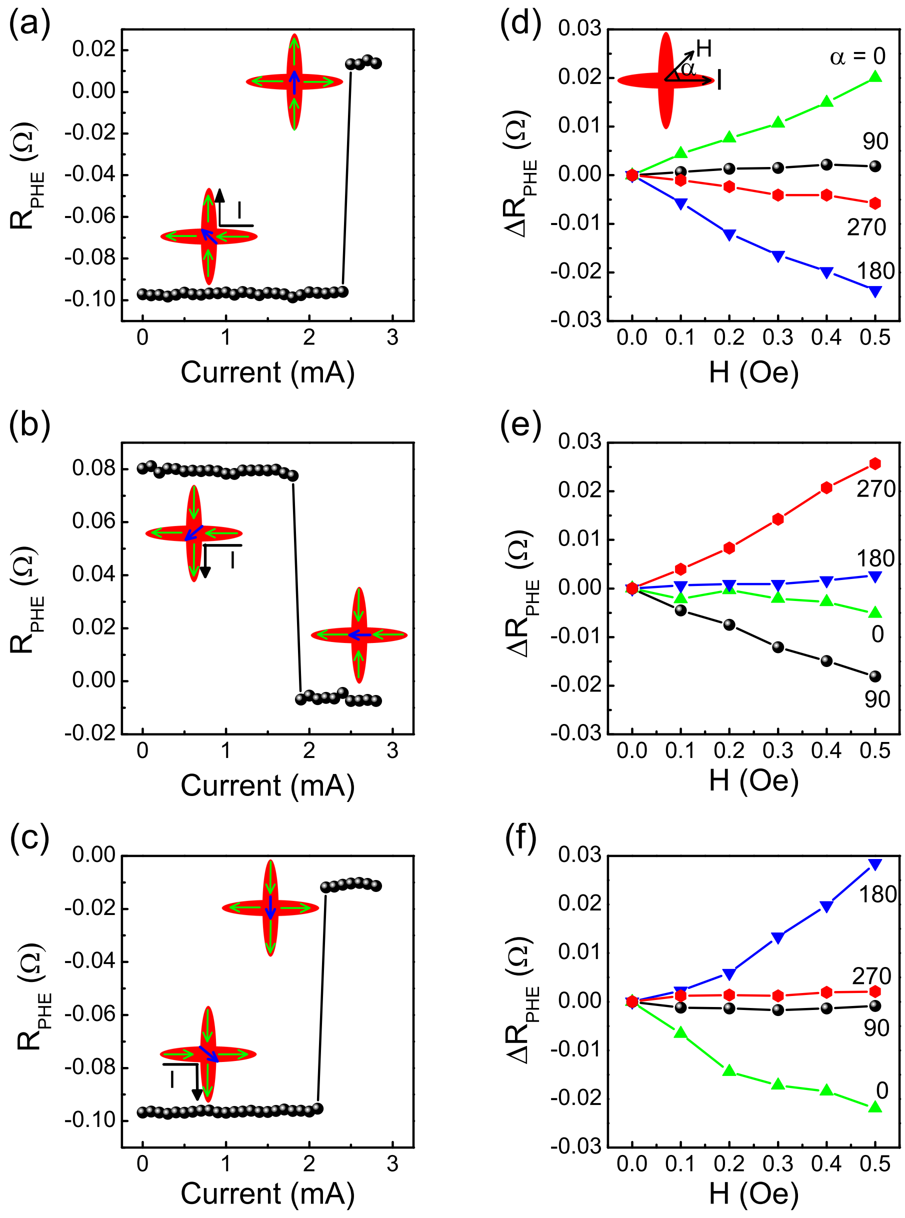


FIG. S6: (a-c) Switchings to NSs, shown in panel F, G and H of Fig. S5 respectively, from OSs by selectively flowing current between the edges of different ellipses. The schematics are showing the direction of magnetization of the edges as well as the overlap area and the current direction. (d-f) Change in $R_{PHE}$ as a function of field at various field directions for three Néel states, respectively.

text. These states are also accessible with SOTs and to distinguish between two states with the same $R_{PHE}$, we can probe their response to external fields (e.g., the direction at which a field should be applied in order to obtain a switching to another OS).

All the states of Group 2 can be achieved experimentally starting from one of the states of Group 1 by flowing current between the edges of different ellipses. For each state we denote in the panel how it can be achieved starting with one of states of Group 1. For example, $A_{32}$ in panel (E) denotes that it can be achieved by flowing a current pulse from pad 3 to pad 2 in state (A). As can be seen there is more than one way to obtain states of Group 2.

Fig. S6(a-c) show switchings to NSs (shown in Fig. S5(F-H), respectively) from three different OSs by flowing current through the edges of different ellipses. The Néel states can be distinguished by measuring their responses to external magnetic field. Fig. S6(d-f) show the change in $R_{PHE}$ as a function of external magnetic field for various field directions in three corresponding NSs, respectively. We clearly observe different responses to external magnetic fields. We note that states that

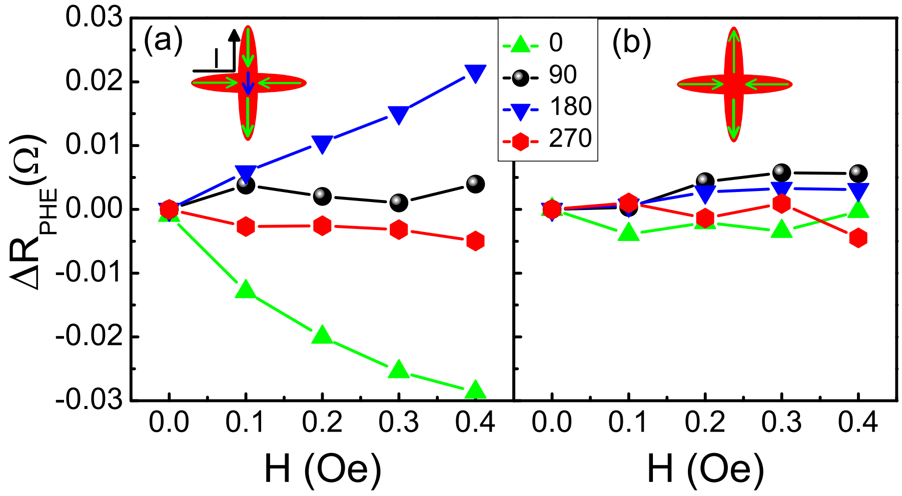


FIG. S7: (a) and (b) $\Delta R_{PHE}$ vs H at various field directions for states in panel (L) Group 2 and panel (N) Group 3, respectively. The state of Group 3 is achieved by flowing current between the edges of different ellipses in Group 2 as shown in the schematics. The schematics also show the direction of magnetization at the edges.

are equivalent in their response to application of a magnetic field at different directions (e.g., states shown in panel (E) and (I)) can be distinguished by the way that they are achieved and the states to which they are switched by applying current through different paths.

The 4 NSs of Group 3 can be achieved experimentally starting from one of the NSs of Group 2 by driving current between the edges of different ellipses. For example, as noted in panel (N), it can be achieved by starting with state (L) and driving current between pads 2 and 3. Fig. S7(a) and (b) show the change in $R_{PHE}$ as a function of field for various directions in states of panel (L) and (N), respectively. The NSs of Group 3 are identified based on their PHE resistance, their negligible response to fields applied at all directions, the way the state was achieved and the states to which it switches in response to currents pulses.

[1] A. Vansteenkiste, J. Leliaert, M. Dvornik, M. Helsen, F. Garcia-Sanchez, and B. V. Waeyenberge, AIP Adv. **4,** 107133 (2014).
